# Supplementary material for: Coexistence of type-I and type-II superconductivity signatures in ZrB12 probed by muon spin rotation measurements
Source: arXiv:1910.09082 source file (2020-10-27)
Supplement: Supplementary file 1 [file SupplementalMaterial_ZrB12.pdf]

# Supplemental Material: Direct evidence of temperature tuned type-I and type-II superconductivity in $\text{ZrB}_{12}$

P. K. Biswas,<sup>1,\*</sup> A. D. Hillier,<sup>1</sup> R. P. Singh,<sup>2</sup> N. Parzyk,<sup>3</sup> G. Balakrishnan,<sup>3</sup>  
M. R. Lees,<sup>3</sup> C. D. Dewhurst,<sup>4</sup> E. Morenzoni,<sup>5,†</sup> and D. M<sup>c</sup>K. Paul<sup>3</sup>

<sup>1</sup>*ISIS Pulsed Neutron and Muon Source, STFC Rutherford Appleton Laboratory,  
Harwell Campus, Didcot, Oxfordshire, OX11 0QX, United Kingdom*

<sup>2</sup>*Indian Institute of Science Education and Research Bhopal, Bhopal, 462066, India*

<sup>3</sup>*Physics Department, University of Warwick, Coventry, CV4 7AL, United Kingdom*

<sup>4</sup>*Institut Laue Langevin, 6 Rue Jules Horowitz, 38042 Grenoble, France*

<sup>5</sup>*Laboratory for Muon Spin Spectroscopy, Paul Scherrer Institut, CH-5232 Villigen PSI, Switzerland*  
(Dated: February 12, 2019)

In this supplemental material we present the sample preparation, magnetic characterisation measurements of the  $\text{ZrB}_{12}$  single crystals using either Quantum Design Magnetic Property Measurement System (MPMS) superconducting quantum interference device (SQUID) magnetometer or an Oxford Instruments (OI) vibrating sample magnetometer (VSM). Details about the experimental methods and data analysis are also presented here.

PACS numbers:

## METHODS

### Single Crystal Growth and Characterisation

Single crystals of  $\text{ZrB}_{12}$  were grown by the floating zone technique in a Crystal Systems Incorporated (CSI) four-mirror infra-red image furnace in a flow of high purity Ar gas at a pressure of 2 bar [1]. The quality of the crystals was checked and the single crystals orientated using x-ray Laue diffraction images.  $\text{ZrB}_{12}$  single crystal made with  $^{11}\text{B}$  isotope to reduce the neutron absorption were grown using a similar method. Pictures of a large single crystal of  $\text{ZrB}_{12}$ , the x-ray Laue-diffraction patterns along different principal axes, and the magnetic characterisation measurements were made using either Quantum Design Magnetic Property Measurement System (MPMS) superconducting quantum interference device (SQUID) magnetometer or an Oxford Instruments (OI) vibrating sample magnetometer (VSM).

### $\mu\text{SR}$ Technique

The  $\mu\text{SR}$  technique makes use of fully polarised positive muons acting as very sensitive local magnetic probes to determine local field distributions within superconducting or magnetic materials. At the ISIS facility, a pulse of muons is produced every 20 ms and has a FWHM of  $\approx 70$  ns. The muons are implanted in the sample where they thermalise at interstitial lattice sites and decay with a lifetime of  $2.2 \mu\text{s}$  into a positron, which is emitted preferentially in the direction of the muon spin direction at the moment of the decay, and two neutrinos. The positrons are detected and time stamped in the detectors placed around the sample. From the collected histograms, the asymmetry in the positron emission as

a function of time  $A(t)$  can be determined, which is directly proportional to the time evolution of the muon spin polarisation.

### Small-Angle Neutron Scattering Technique

Small-angle neutron scattering measurements were performed using the D22 instrument at the Institut Laue-Langevin, Grenoble, France. D22 was configured in a high-resolution mode with a mean wavelength of  $10 \text{ \AA}$ , wavelength spread of 10%, and collimation of  $17.6 \text{ m}$ . An additional circular aperture of diameter  $20 \text{ mm}$  was also used before the sample to better define the scattered beam at the detector and to equalise the horizontal and vertical divergences. Diffracted neutrons were collected with a position-sensitive two-dimensional multidetector located  $17.6 \text{ m}$  after the sample. The samples were mounted with the  $a$ -axis parallel to the neutron beam direction to access the Bragg peaks. To scan through the Bragg condition for a diffraction spot, a rocking curve was performed by tilting or rotating the sample, cryostat, and magnet together about a horizontal or vertical axis. For all measurements, the sample was cooled to the base temperature in an applied magnetic field  $H$  and the data collected while warming the sample in the same field. Background scattering was measured above  $T_c$  and subtracted from the low-temperature data.

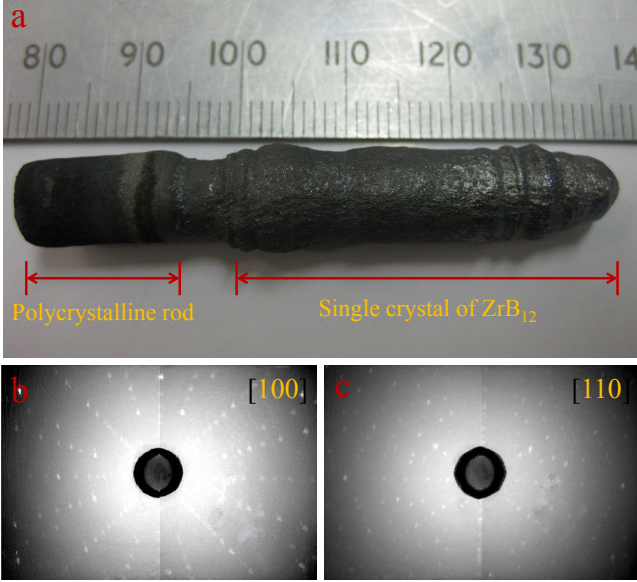

FIG. S1: **Single crystal and Laue patterns of  $\text{ZrB}_{12}$ .** **a** Single crystal of  $\text{ZrB}_{12}$  grown using the floating zone method in a four mirror optical image furnace. **b** and **c** Typical x-ray Laue back-reflection patterns obtained from a crystal of  $\text{ZrB}_{12}$ . The images were taken with the x-rays directed along the  $[100]$  (parallel the  $a$ -axis) and the  $[110]$  directions.

## SAMPLE PREPARATION AND CHARACTERISATION

### Single Crystals of $\text{ZrB}_{12}$

Figure S1 (a) shows a large single crystal of  $\text{ZrB}_{12}$ , grown using the floating zone method. The crystal quality was checked and the samples orientated using the x-ray Laue technique. Images of the x-ray Laue-diffraction patterns along the  $[100]$  and  $[110]$  directions are shown in Figs. S1 (b) and (c).

### Sample Preparation

A large single crystal of  $\text{ZrB}_{12}$  was cut into several disc-shaped pieces of thickness 1.5-2 mm and diameter 4-5 mm, all having the same crystallographic orientation with the  $c$ -axis perpendicular to the disc's plane. The sample used for the muon experiments was a mosaic of seven such single-crystal discs with the crystallographic  $c$ -axis parallel to the incident muon beam. The crystals were mounted onto a 99.995% pure silver plate. Thin haematite ( $\text{Fe}_2\text{O}_3$ ) slabs were positioned immediately behind the sample. The muons stopping in the  $\text{Fe}_2\text{O}_3$  slabs depolarise very quickly thus suppressing the background signal significantly.

### Sample Characterisation

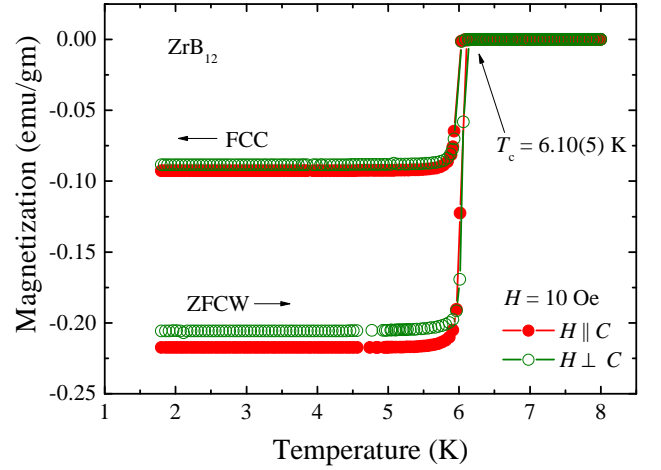

FIG. S2: **Magnetisation vs temperature for  $\text{ZrB}_{12}$ .** Temperature dependence of the dc magnetisation of  $\text{ZrB}_{12}$  measured on zero-field-cooled warming (ZFCW) and field-cooled cooling (FCC). The magnetic field was applied parallel and perpendicular to the  $c$ -axis. The diamagnetic susceptibility shows a  $T_c$  onset at  $6.10(5)$  K.

The temperature dependence of the magnetisation of  $\text{ZrB}_{12}$  was measured using a Quantum Design MPMS magnetometer. A field of 10 Oe was applied parallel and perpendicular to the  $c$ -axis. Data were taken in both zero-field-cooled warming and the field-cooled cooling modes. The samples has a superconducting transition temperature  $T_c$  of  $(6.10 \pm 0.05)$  K. The diamagnetic response is isotropic.

Magnetisation measurements were performed as a function of applied field. Figure S3 shows the virgin magnetisation curves of the sample  $\text{ZrB}_{12}$  taken at different fixed temperatures. At low temperatures, we see a deviation from linearity of the  $M(H)$  curves as the magnetisation approaches zero. Such a deviation indicates that the applied field enters the material in the form of vortex lattice, a characteristic signature of a type-II superconductor. Red dashed lines have been used as an extrapolation of the linear behaviour of  $M(H)$  to  $M = 0$  and also act as a guide to the eye to identify the deviation more clearly. For temperatures close to  $T_c$ , the  $M(H)$  curves exhibit a behaviour more typical of a type-I superconductor as the magnetisation sharply approaches zero at the critical field (see e.g. the 5.5 K data).

Figure S4 shows the temperature dependence of the thermodynamic critical field ( $H_c$ ) and upper critical field ( $H_{c2}$ ) of  $\text{ZrB}_{12}$ . At each temperature  $H_c$  was estimated from the linear extrapolation (dashed lines) of the  $M(H)$  curves to  $M = 0$ . We define  $H_{c2}$  as the field at which the sample enters the normal state. We fit the temper-

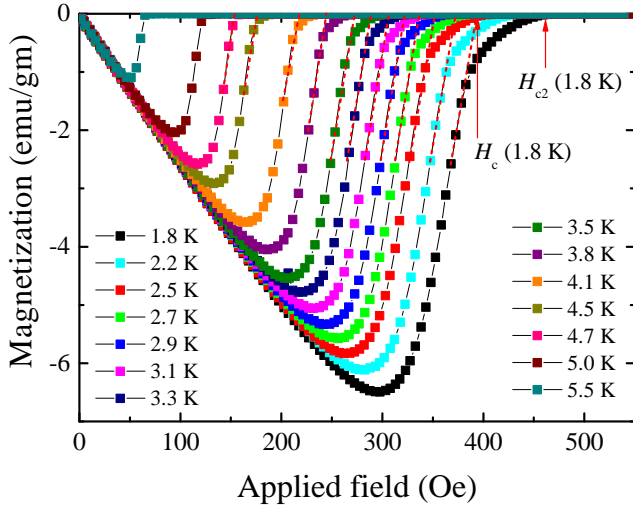

FIG. S3: **Magnetisation vs applied field for ZrB<sub>12</sub>.** Virgin magnetisation curves for a single crystal sample of ZrB<sub>12</sub> taken at different fixed temperatures. Red dashed lines are a guide to the eye to identify the deviation from linearity of the  $M(H)$  curves as the signal approaches  $M = 0$ .

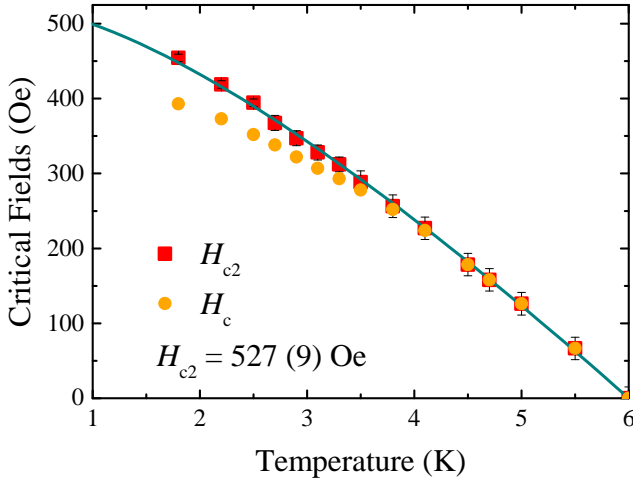

FIG. S4: **Critical fields for ZrB<sub>12</sub>.** Temperature dependence of the thermodynamic critical field ( $H_c$ ) and upper critical field ( $H_{c2}$ ) of ZrB<sub>12</sub>, estimated from the  $M(H)$  data. The data indicate a transition from type-I to type-II behaviour around 4 K.

ature dependence of the  $H_{c2}$  data using the Werthamer-Helfand-Hohenberg model to estimate the value of the critical field of ZrB<sub>12</sub> at  $T=0$  K. The fit yields  $H_{c2}(0) = 527(9)$  Oe.

#### $\mu$ SR Data Analysis

The  $\mu$ SR measurements were performed with a magnetic field transverse to the initial muon spin polarization. The TF time spectra were analysed using the following oscillatory decaying Gaussian function:

$$G_x(t) = A_{bg} \cos(2\pi\nu_{bg} + \phi) + A_{0Meiss} \left[ \frac{1}{3} + \frac{2}{3} (1 - \sigma_{KT}^2 t^2) \exp\left(-\frac{\sigma_{KT}^2 t^2}{2}\right) \right] + \sum_{i=\text{inter, mix}} A_{0i} \exp\left(-\frac{\sigma_i^2 t^2}{2}\right) \cos(2\pi\nu_i + \phi), \quad (\text{S1})$$

where the  $A_{bg} \cos(2\pi\nu_{bg} + \phi)$  term represents the muons

implanted into the silver plate supporting the ZrB<sub>12</sub> sam-

ple, the Kubo-Toyabe (KT) term is present to account for the static response of the Zr nuclear moments in the Meissner phase and the summation allows the inclusion of Gaussian distributions of magnetic fields representing the intermediate or mixed states.

#### Quantitative analysis of the $\mu$ SR data:

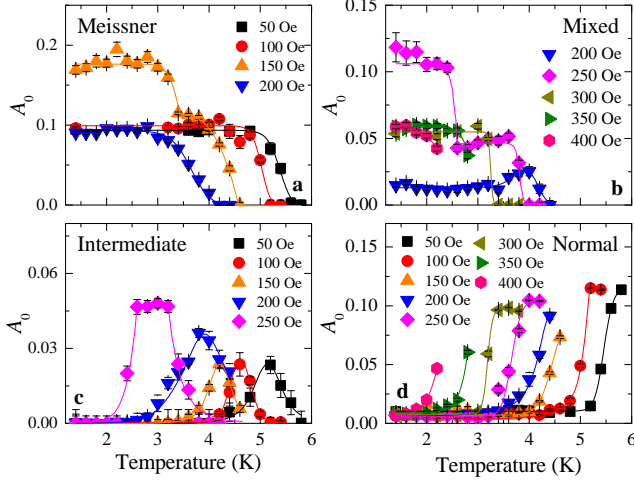

FIG. S5: **TF- $\mu$ SR signals in  $\text{ZrB}_{12}$ .** Temperature dependence of the initial asymmetry  $A_0$  of the  $\mu$ SR time spectra for various applied fields for the **a** Meissner, **b** mixed, **c** intermediate and **d** normal states.  $A_0(T)$  has been extracted by fitting the TF- $\mu$ SR time spectra using Eq. S1.

Figures S5 **a**, **b**, **c**, and **d** show the temperature dependence of the initial asymmetry  $A_0$  of the TF- $\mu$ SR time spectra for different applied fields for the **a** Meissner, **b** mixed, **c** intermediate and **d** normal states. The temperature dependence of  $A_0$  were extracted by fitting the TF- $\mu$ SR time spectra using Eq. S1. Plots of  $A_0$  vs temperature show the variation of the volume fraction of a particular superconducting phase with temperature at different applied fields. Solid lines are guides to the eye. In all cases, the appearance of the different superconducting phases shifts to lower temperature with increasing field.

\* pabitra.biswas@stfc.ac.uk

† Electronic address: elvezio.morenzoni@psi.ch

[1] Balakrishnan, G., Lees, M. R. & Paul, D. M. Growth of large single crystals of rare earth hexaborides. *J. Crystal Growth* **256**, 206209 (2003).
